# Supplementary material for: Bayesian learning of COVID-19 Vaccine safety while incorporating Adverse Events ontology
Source: arXiv:2202.05370 ancillary file (2022-02-10)
Supplement: Supplementary file 1 [file B_gibbs.pdf]

# Mathematical Details of the Gibbs Sampler

Let  $\Theta$  denote the vector form of all the parameters in our model including  $\beta_j^{**}$ 's,  $\sigma_{\beta,j}$ 's,  $\delta_j$ 's,  $\alpha_j$ 's,  $\tau^2$ ,  $\sigma_{\alpha,l}$ 's, and the augmented polya-gamma variables  $\omega_{ij}$ 's. Let  $\mathbf{D}$  denote the observed data, i.e.,  $A_{ij}$ 's. Finally, the full posterior likelihood of  $\Theta$  can be written as equation 1.

$$\begin{aligned}
 \pi(\Theta \mid \mathbf{D}) &\propto \prod_{i=1}^n \prod_{j=1}^J \exp \left\{ -\frac{\omega_{ij} \psi_{ij}^2}{2} + (A_{ij} - 1/2) \psi_{ij} \right\} f_{PG(1,0)}(\omega_{ij}) \\
 &\times \prod_{j=1}^J \prod_{l=0}^p (\sigma_{\alpha,l}^2)^{-1/2} \exp \left( -\frac{\alpha_{jl}^2}{2\sigma_{\alpha,l}^2} \right) \times \prod_{l=0}^p (\sigma_{\alpha,l}^2)^{-a_{\alpha}-1} \exp \left( -\frac{b_{\alpha}}{\sigma_{\alpha,l}^2} \right) \\
 &\times |\Omega_{\epsilon}|^{-1/2} \exp \left\{ -\frac{1}{2} \beta^{**\top} \Omega_{\epsilon}^{-1} \beta^{**} \right\} \\
 &\times \prod_{j=1}^J (\tau^2)^{-1/2} \exp \left\{ -\frac{\sigma_{\beta,j}^2}{2\tau^2} \right\} \times (\tau^2)^{-a_{\tau}-1} \exp \left( \frac{b_{\tau}}{\tau^2} \right) \\
 &\times \prod_{j=1}^J \pi^{\delta_j} (1 - \pi)^{1-\delta_j}
 \end{aligned} \tag{1}$$

Here  $\psi_{ij} = \mathbf{X}_i^{\top} \alpha_j + \delta_j \beta_j^{**} \sigma_{\beta,j} V_i$ .

For notational simplicity, we define  $\cdot \mid \text{rest}$  to be the posterior conditional distribution of  $\cdot$  given all the rest of parameters in  $\Theta$ .

The full conditional distribution of  $\omega_{ij}$  is given by

$$\omega_{ij} \mid \text{rest} \sim \text{PG}(1, \psi_{ij}) \tag{2}$$

The full conditional distribution of  $\alpha_j$  is given by

$$\begin{aligned}
 \alpha_j \mid \text{rest} &\sim \text{N}(\mu_{\alpha,j}, \Sigma_{\alpha,j}) \\
 \mu_{\alpha,j} &= \Sigma_{\alpha,j} \mathbf{X}^{\top} \left( \mathbf{A}_j - \frac{1}{2} \mathbf{1}_n - \beta_j \Omega_j \mathbf{V} \right) \\
 \Sigma_{\alpha,j} &= \left( \mathbf{X}^{\top} \Omega_j \mathbf{X} + \text{diag} \left\{ \frac{1}{\sigma_{\alpha 0}^2}, \dots, \frac{1}{\sigma_{\alpha p}^2} \right\} \right)^{-1}
 \end{aligned} \tag{3}$$

where  $\mathbf{A}_j = (A_{1j}, \dots, A_{nj})^\top$ ,  $\mathbf{\Omega}_j = \text{diag}(\omega_{1j}, \dots, \omega_{nj})$ , and  $\mathbf{V} = (V_1, \dots, v_n)^\top$ .

The full conditional distribution of  $\beta_j^{**}$  is given by

$$\begin{aligned}\beta_j^{**} \mid \text{rest} &\sim N(\mu_{\beta,j}, \sigma_{\beta^{**},j}^2) \\ \mu_{\beta,j} &= \sigma_{\beta^{**},j}^2 \left( \sigma_{\beta,j} \delta_j (\mathbf{A}_j^\top - \frac{1}{2} \mathbf{1}_n^\top - \boldsymbol{\alpha}_j^\top \mathbf{X}^\top \mathbf{\Omega}_j) \mathbf{V} - \sum_{j \neq k} \beta_k^{**} \rho_{jk}^* \right) \\ \sigma_{\beta^{**},j}^2 &= (\sigma_{\beta,j}^2 \delta_j \mathbf{V}^\top \mathbf{\Omega}_j \mathbf{V} + \rho_{jj}^*)^{-1}\end{aligned}\tag{4}$$

Here  $\rho_{jk}^*$  is the  $(j, k)$ -th element of  $\mathbf{\Omega}_\epsilon^{-1}$ .

The full conditional distribution of  $\sigma_{\beta,j}$  is given by

$$\begin{aligned}\sigma_{\beta,j} \mid \text{rest} &\sim FN(\mu_{\sigma,j}, \sigma_{\sigma,j}^2) \\ \mu_{\sigma,j} &= \sigma_{\sigma,j}^2 \beta_j^{**} \delta_j (\mathbf{A}_j^\top - \frac{1}{2} \mathbf{1}_n^\top - \boldsymbol{\alpha}_j^\top \mathbf{X}^\top \mathbf{\Omega}_j) \mathbf{V} \\ \sigma_{\sigma,j}^2 &= \left( \beta_j^{**2} \delta_j \mathbf{V}^\top \mathbf{\Omega}_j \mathbf{V} + \frac{1}{\tau^2} \right)^{-1}\end{aligned}\tag{5}$$

The full conditional distribution of  $\sigma_{\alpha,l}^2$  is given by

$$\sigma_{\alpha,l}^2 \mid \text{rest} \sim \text{IG} \left( a_\alpha + \frac{J}{2}, b_\alpha + \frac{1}{2} \sum_{j=1}^J \alpha_{jl}^2 \right)\tag{6}$$

The full conditional distribution of  $\tau^2$  is given by

$$\tau^2 \mid \text{rest} \sim \text{IG} \left( a_\tau + \frac{J}{2}, b_\tau + \frac{1}{2} \sum_{j=1}^J \sigma_{\beta,j}^2 \right)\tag{7}$$

The full conditional distribution of  $\delta_j$  is given by

$$\begin{aligned}\delta_j &\sim \text{Bern} \left( \frac{1}{1 + \frac{1-\pi}{\pi} \exp(-D_j)} \right) \\ D_j &= \sigma_{\beta,j} \beta_j^{**} (\mathbf{A}_j^\top - \frac{1}{2} \mathbf{1}_n^\top - \boldsymbol{\alpha}_j^\top \mathbf{X}^\top \mathbf{\Omega}_j) \mathbf{V} - \frac{1}{2} \sigma_{\beta,j}^2 \beta_j^{**2} \mathbf{V}^\top \mathbf{\Omega}_j \mathbf{V}\end{aligned}\tag{8}$$
