# Supplementary material for: Bayesian learning of COVID-19 Vaccine safety while incorporating Adverse Events ontology
Source: arXiv:2202.05370 ancillary file (2022-02-10)
Supplement: Supplementary file 2 [file D_Study2_MP_JJ.pdf]

## AE signals in Study II (Pfizer–BioNTech and Moderna vs Johnson & Johnson–Janssen)

In the following tables, **AE\_NAME** is the name of the AE; **beta** is the log odds ratio of the occurrence of the AE of mRNA-based vaccines to J & J; **beta\_upper** and **beta\_lower** are the boundaries of 95% credit intervals; The **inclusion\_prob** is the inclusion probabilities of the AE, i.e.,  $\delta_j$ ; **n\_MP** and **n\_JJ** are the numbers of occurrences of the AE in reports on mRNA-based vaccines and J & J respectively.

Total number of reports:  $5.88487 \times 10^5$  ( $5.3939 \times 10^5$  for mRNA-based vaccines and  $4.9097 \times 10^4$  for J & J)

### AEs with increased risk in mRNA-based COVID-19 vaccines compared to J & J

| AE_NAME                                          | beta | beta_lower | beta_upper | inclusion_prob | n_MP  | n_JJ |
|--------------------------------------------------|------|------------|------------|----------------|-------|------|
| Vaccination site swelling                        | 3.05 | 2.87       | 3.19       | 1              | 4843  | 14   |
| Vaccination site pain                            | 2.74 | 2.44       | 3.02       | 1              | 12748 | 60   |
| Vaccine positive rechallenge                     | 2.31 | 1.83       | 2.65       | 1              | 1687  | 10   |
| Injection site rash                              | 1.95 | 1.75       | 2.13       | 1              | 10384 | 125  |
| Injection site pruritus                          | 1.88 | 1.77       | 2.00       | 1              | 18573 | 235  |
| Immunisation                                     | 1.84 | 1.64       | 2.02       | 1              | 1886  | 27   |
| Maternal exposure during pregnancy               | 1.70 | 1.27       | 2.04       | 1              | 834   | 14   |
| Inappropriate schedule of product administration | 1.63 | 1.50       | 1.85       | 1              | 6721  | 129  |
| Injection site urticaria                         | 1.62 | 1.31       | 1.91       | 1              | 1370  | 23   |
| Myocarditis                                      | 1.52 | 1.19       | 1.74       | 1              | 1537  | 53   |
| Injection site warmth                            | 1.43 | 1.33       | 1.56       | 1              | 13597 | 261  |
| Injection site erythema                          | 1.43 | 1.33       | 1.50       | 1              | 26459 | 542  |
| Injection site induration                        | 1.28 | 1.13       | 1.43       | 1              | 5144  | 110  |
| Lymphadenopathy                                  | 1.19 | 1.11       | 1.29       | 1              | 19083 | 557  |
| Lymph node pain                                  | 1.16 | 1.01       | 1.37       | 1              | 4497  | 133  |
| Axillary pain                                    | 1.15 | 0.98       | 1.33       | 1              | 5062  | 150  |
| Axillary mass                                    | 1.14 | 0.83       | 1.50       | 1              | 711   | 17   |
| Injection site reaction                          | 1.12 | 0.95       | 1.29       | 1              | 4236  | 122  |
| Skin reaction                                    | 1.07 | 0.67       | 1.41       | 1              | 635   | 19   |
| Injection site swelling                          | 1.03 | 0.96       | 1.10       | 1              | 21526 | 665  |
| Lymphadenitis                                    | 0.97 | 0.48       | 1.44       | 1              | 277   | 10   |
| Tongue pruritus                                  | 0.84 | 0.57       | 1.14       | 1              | 464   | 17   |
| Product storage error                            | 0.83 | 0.73       | 0.94       | 1              | 9014  | 421  |
| Rash erythematous                                | 0.83 | 0.71       | 0.94       | 1              | 9233  | 338  |
| Incorrect route of product administration        | 0.81 | 0.59       | 1.04       | 1              | 775   | 34   |
| Injection site inflammation                      | 0.79 | 0.55       | 1.03       | 1              | 950   | 33   |
| Rash papular                                     | 0.78 | 0.63       | 0.93       | 1              | 2862  | 112  |
| Erythema                                         | 0.74 | 0.66       | 0.81       | 1              | 20503 | 804  |
| Incorrect product formulation administered       | 0.71 | 0.39       | 1.02       | 1              | 639   | 30   |

### AEs with increased risk in J & J compared to mRNA-based COVID-19 vaccines

| AE_NAME                                 | beta  | beta_lower | beta_upper | inclusion_prob | n_MP | n_JJ |
|-----------------------------------------|-------|------------|------------|----------------|------|------|
| Urinary retention                       | -0.69 | -0.97      | -0.44      | 1.00           | 200  | 35   |
| Type 2 diabetes mellitus                | -0.70 | -1.08      | -0.35      | 1.00           | 110  | 18   |
| Renal pain                              | -0.70 | -0.91      | -0.46      | 1.00           | 532  | 100  |
| Cerebral infarction                     | -0.70 | -1.07      | -0.50      | 1.00           | 225  | 38   |
| Fine motor skill dysfunction            | -0.70 | -1.13      | -0.24      | 1.00           | 126  | 25   |
| Cerebrovascular accident                | -0.71 | -0.81      | -0.57      | 1.00           | 2308 | 334  |
| Vision blurred                          | -0.72 | -0.79      | -0.65      | 1.00           | 5239 | 1022 |
| Piloerection                            | -0.72 | -1.05      | -0.41      | 1.00           | 116  | 26   |
| Rectal haemorrhage                      | -0.74 | -1.17      | -0.41      | 1.00           | 215  | 34   |
| Atypical pneumonia                      | -0.74 | -1.15      | -0.46      | 1.00           | 78   | 11   |
| Urinary incontinence                    | -0.74 | -0.94      | -0.52      | 1.00           | 672  | 125  |
| Feeling cold                            | -0.74 | -0.81      | -0.66      | 1.00           | 5372 | 1012 |
| Intensive care                          | -0.74 | -0.87      | -0.60      | 1.00           | 1655 | 284  |
| Incoherent                              | -0.74 | -1.04      | -0.39      | 1.00           | 218  | 42   |
| Loss of consciousness                   | -0.74 | -0.80      | -0.69      | 1.00           | 7367 | 1735 |
| Hypophagia                              | -0.75 | -0.98      | -0.51      | 1.00           | 446  | 65   |
| Fluid intake reduced                    | -0.75 | -1.13      | -0.34      | 1.00           | 103  | 17   |
| Nail discolouration                     | -0.75 | -1.19      | -0.23      | 1.00           | 63   | 17   |
| Restless legs syndrome                  | -0.75 | -1.00      | -0.48      | 1.00           | 218  | 42   |
| CIDP                                    | -0.76 | -1.12      | -0.49      | 1.00           | 39   | 11   |
| Fear of injection                       | -0.76 | -1.01      | -0.52      | 1.00           | 213  | 65   |
| Hemiparesis                             | -0.77 | -0.97      | -0.56      | 1.00           | 664  | 118  |
| Haemoptysis                             | -0.77 | -0.96      | -0.55      | 1.00           | 317  | 65   |
| Peripheral artery thrombosis            | -0.77 | -1.22      | -0.40      | 1.00           | 53   | 13   |
| Endotracheal intubation                 | -0.77 | -0.92      | -0.59      | 1.00           | 963  | 161  |
| Contusion                               | -0.77 | -0.87      | -0.68      | 1.00           | 3043 | 551  |
| Apathy                                  | -0.77 | -1.20      | -0.49      | 1.00           | 71   | 16   |
| Haemorrhagic stroke                     | -0.77 | -1.26      | -0.48      | 1.00           | 86   | 12   |
| Snoring                                 | -0.78 | -1.28      | -0.43      | 1.00           | 65   | 18   |
| Increased tendency to bruise            | -0.78 | -1.30      | -0.23      | 1.00           | 45   | 12   |
| Groin pain                              | -0.78 | -1.02      | -0.55      | 1.00           | 388  | 67   |
| Eye movement disorder                   | -0.79 | -0.98      | -0.63      | 1.00           | 608  | 162  |
| Respiratory failure                     | -0.79 | -1.02      | -0.56      | 1.00           | 521  | 80   |
| Sensory disturbance                     | -0.80 | -0.98      | -0.65      | 1.00           | 811  | 168  |
| Acute respiratory distress syndrome     | -0.80 | -1.23      | -0.43      | 1.00           | 154  | 29   |
| Anticoagulant therapy                   | -0.80 | -0.92      | -0.69      | 1.00           | 1699 | 317  |
| Acute respiratory failure               | -0.81 | -0.97      | -0.64      | 1.00           | 1280 | 184  |
| Bladder catheterisation                 | -0.82 | -1.22      | -0.46      | 1.00           | 98   | 15   |
| Haematemesis                            | -0.84 | -1.21      | -0.57      | 1.00           | 156  | 35   |
| Psychomotor hyperactivity               | -0.85 | -1.12      | -0.56      | 1.00           | 86   | 15   |
| Plasmapheresis                          | -0.86 | -1.37      | -0.41      | 1.00           | 77   | 19   |
| Gastrointestinal tube insertion         | -0.87 | -1.17      | -0.46      | 1.00           | 59   | 11   |
| Hypoxia                                 | -0.87 | -0.99      | -0.75      | 1.00           | 1746 | 271  |
| Extubation                              | -0.88 | -1.41      | -0.40      | 1.00           | 50   | 11   |
| Dysaesthesia                            | -0.88 | -1.43      | -0.42      | 1.00           | 40   | 10   |
| Hypotonia                               | -0.89 | -1.22      | -0.62      | 1.00           | 168  | 41   |
| Cerebral thrombosis                     | -0.90 | -1.30      | -0.43      | 1.00           | 140  | 30   |
| Cerebral small vessel ischaemic disease | -0.91 | -1.44      | -0.49      | 1.00           | 92   | 15   |
| Rhinalgia                               | -0.91 | -1.38      | -0.42      | 1.00           | 71   | 17   |
| Ischaemic stroke                        | -0.94 | -1.19      | -0.64      | 1.00           | 275  | 56   |
| Mesenteric vein thrombosis              | -0.95 | -1.25      | -0.51      | 1.00           | 40   | 12   |
| Tension                                 | -0.96 | -1.31      | -0.63      | 1.00           | 164  | 46   |

| AE_NAME                            | beta  | beta_lower | beta_upper | inclusion_prob | n_MP | n_JJ |
|------------------------------------|-------|------------|------------|----------------|------|------|
| Overdose                           | -0.97 | -1.37      | -0.68      | 1.00           | 163  | 46   |
| Vaccination failure                | -0.97 | -1.14      | -0.75      | 1.00           | 581  | 151  |
| Pulmonary embolism                 | -1.00 | -1.09      | -0.91      | 1.00           | 2377 | 542  |
| Fluid replacement                  | -1.00 | -1.45      | -0.66      | 1.00           | 31   | 10   |
| Jugular vein thrombosis            | -1.01 | -1.39      | -0.62      | 1.00           | 39   | 12   |
| Thrombocytopenia                   | -1.02 | -1.21      | -0.83      | 1.00           | 499  | 115  |
| Affect lability                    | -1.02 | -1.57      | -0.60      | 1.00           | 34   | 9    |
| Thrombectomy                       | -1.03 | -1.28      | -0.82      | 1.00           | 207  | 50   |
| Posture abnormal                   | -1.04 | -1.28      | -0.85      | 1.00           | 231  | 72   |
| New daily persistent headache      | -1.05 | -1.56      | -0.52      | 1.00           | 41   | 14   |
| Carotid artery thrombosis          | -1.05 | -1.71      | -0.47      | 1.00           | 22   | 10   |
| Platelet transfusion               | -1.05 | -1.39      | -0.79      | 1.00           | 117  | 30   |
| Carotid artery occlusion           | -1.06 | -1.64      | -0.47      | 1.00           | 37   | 11   |
| Pulmonary thrombosis               | -1.06 | -1.28      | -0.85      | 1.00           | 450  | 101  |
| Immunoglobulin therapy             | -1.06 | -1.29      | -0.83      | 1.00           | 401  | 110  |
| Carotid artery stenosis            | -1.06 | -1.52      | -0.47      | 1.00           | 42   | 11   |
| Poor peripheral circulation        | -1.06 | -1.49      | -0.57      | 1.00           | 88   | 24   |
| General symptom                    | -1.07 | -1.50      | -0.71      | 1.00           | 37   | 12   |
| Emphysema                          | -1.07 | -1.47      | -0.74      | 1.00           | 71   | 15   |
| Muscle contracture                 | -1.07 | -1.38      | -0.79      | 1.00           | 81   | 23   |
| Capillary fragility                | -1.08 | -1.38      | -0.72      | 1.00           | 28   | 11   |
| Bilevel positive airway pressure   | -1.08 | -1.49      | -0.53      | 1.00           | 155  | 33   |
| Acute left ventricular failure     | -1.09 | -1.69      | -0.60      | 1.00           | 50   | 10   |
| Vein disorder                      | -1.10 | -1.54      | -0.79      | 1.00           | 100  | 27   |
| Foaming at mouth                   | -1.10 | -1.49      | -0.77      | 1.00           | 77   | 22   |
| Subarachnoid haemorrhage           | -1.11 | -1.58      | -0.62      | 1.00           | 107  | 24   |
| Mechanical ventilation             | -1.12 | -1.33      | -0.92      | 1.00           | 467  | 104  |
| Thrombosis                         | -1.13 | -1.21      | -1.04      | 1.00           | 2524 | 675  |
| Deep vein thrombosis               | -1.19 | -1.30      | -1.10      | 1.00           | 1691 | 472  |
| Thrombophlebitis                   | -1.20 | -1.62      | -0.70      | 1.00           | 39   | 12   |
| Cerebral haemorrhage               | -1.21 | -1.43      | -1.01      | 1.00           | 299  | 74   |
| Varicose vein                      | -1.21 | -1.62      | -0.72      | 1.00           | 79   | 26   |
| Transverse sinus thrombosis        | -1.21 | -1.84      | -0.63      | 1.00           | 41   | 16   |
| Superior sagittal sinus thrombosis | -1.22 | -1.91      | -0.59      | 1.00           | 28   | 11   |
| Cerebral artery occlusion          | -1.22 | -1.70      | -0.85      | 1.00           | 53   | 17   |
| Craniocerebral injury              | -1.22 | -1.74      | -0.84      | 1.00           | 32   | 12   |
| Vasodilatation                     | -1.30 | -1.54      | -1.08      | 1.00           | 109  | 36   |
| Guillain-Barre syndrome            | -1.35 | -1.50      | -1.13      | 1.00           | 512  | 178  |
| Portal vein thrombosis             | -1.35 | -1.67      | -0.97      | 1.00           | 58   | 24   |
| Embolic stroke                     | -1.39 | -2.20      | -1.05      | 1.00           | 43   | 14   |
| Thrombophlebitis superficial       | -1.43 | -1.73      | -1.17      | 1.00           | 129  | 51   |
| Venous occlusion                   | -1.43 | -2.32      | -0.90      | 1.00           | 19   | 10   |
| Coronary artery thrombosis         | -1.44 | -2.31      | -0.86      | 1.00           | 41   | 12   |
| Cerebral venous thrombosis         | -1.45 | -1.85      | -0.93      | 1.00           | 27   | 12   |
| Gaze palsy                         | -1.46 | -1.69      | -1.26      | 1.00           | 191  | 82   |
| Intracardiac thrombus              | -1.47 | -1.93      | -1.00      | 1.00           | 67   | 24   |
| Sick relative                      | -1.51 | -1.97      | -1.05      | 1.00           | 35   | 11   |
| Craniotomy                         | -1.53 | -2.07      | -0.81      | 1.00           | 30   | 11   |
| Embolism                           | -1.58 | -2.01      | -1.18      | 1.00           | 30   | 12   |
| Spider vein                        | -1.73 | -2.28      | -1.16      | 1.00           | 17   | 10   |
| Tracheostomy                       | -1.76 | -2.35      | -1.20      | 1.00           | 27   | 12   |
| Haemorrhoids thrombosed            | -1.86 | -2.48      | -1.35      | 1.00           | 14   | 11   |

| AE_NAME               | beta  | beta_lower | beta_upper | inclusion_prob | n_MP | n_JJ |
|-----------------------|-------|------------|------------|----------------|------|------|
| Peripheral embolism   | -2.25 | -2.86      | -1.54      | 1.00           | 15   | 17   |
| On and off phenomenon | -2.37 | -3.01      | -1.96      | 1.00           | 17   | 16   |
| Therapy non-responder | -4.38 | -4.80      | -4.09      | 1.00           | 22   | 121  |
| Pneumonia viral       | -0.70 | -1.34      | 0.00       | 0.94           | 91   | 14   |

## Enriched AE groups and signals within enriched groups

It is also worth looking at which AE signals were indentified within enriched groups.

|                                                                                                                                                                                                                                                                                                                                                                                                                                                                                      |
|--------------------------------------------------------------------------------------------------------------------------------------------------------------------------------------------------------------------------------------------------------------------------------------------------------------------------------------------------------------------------------------------------------------------------------------------------------------------------------------|
| Administration Site Reactions (Enriched Group for mRNA vaccines)                                                                                                                                                                                                                                                                                                                                                                                                                     |
| Vaccination site swelling, Vaccination site pain, Injection site rash, Injection site pruritus, Injection site urticaria, Injection site warmth, Injection site erythema, Injection site induration, Injection site reaction, Injection site swelling, Injection site inflammation                                                                                                                                                                                                   |
| Embolism and thrombosis (Enriched Group for J & J)                                                                                                                                                                                                                                                                                                                                                                                                                                   |
| Peripheral artery thrombosis, Cerebral thrombosis, Mesenteric vein thrombosis, Pulmonary embolism, Jugular vein thrombosis, Carotid artery thrombosis, Pulmonary thrombosis, Thrombosis, Deep vein thrombosis, Thrombophlebitis, Transverse sinus thrombosis, Superior sagittal sinus thrombosis, Portal vein thrombosis, Embolic stroke, Thrombophlebitis superficial, Coronary artery thrombosis, Cerebral venous thrombosis, Intracardiac thrombus, Embolism, Peripheral embolism |
| Central nervous system vascular disorders (Enriched Group for J & J)                                                                                                                                                                                                                                                                                                                                                                                                                 |
| Cerebral infarction, Cerebrovascular accident, Haemorrhagic stroke, Cerebral thrombosis, Cerebral small vessel ischaemic disease, Ischaemic stroke, Carotid artery thrombosis, Carotid artery occlusion, Carotid artery stenosis, Subarachnoid haemorrhage, Cerebral haemorrhage, Transverse sinus thrombosis, Superior sagittal sinus thrombosis, Cerebral artery occlusion, Embolic stroke, Cerebral venous sinus thrombosis                                                       |
