# Supplementary material for: Bayesian learning of COVID-19 Vaccine safety while incorporating Adverse Events ontology
Source: arXiv:2202.05370 ancillary file (2022-02-10)
Supplement: Supplementary file 3 [file E_comparison.pdf]

# Comparison of GPS and BGrass on Real Data

We applied the GPS model on real data studies to compare the results with our BGrass model. The R package we used was **openEBGM**. GPS computes an quantity named *EBGM* to identify signals. We set the criteria of signals to be the 1% quantile of the posterior distribution of *ebgm* being greater than 1. We've made a Venn diagram and a table for displaying signals discovered by GPS, BGrass, and both.

## The initial value for hyper parameters:

We used five initial values, all of them converged to the same estimator eventually.

| alpha1 | beta1 | alpha2 | beta2 | p    |
|--------|-------|--------|-------|------|
| 0.2    | 0.1   | 2      | 4     | 0.33 |
| 0.1    | 0.1   | 10     | 10    | 0.20 |
| 0.3    | 0.5   | 6      | 6     | 0.50 |
| 0.5    | 0.3   | 12     | 12    | 0.80 |
| 0.2    | 0.2   | 5      | 5     | 0.40 |

## Study I

| Estimate |         |
|----------|---------|
| alpha1   | 0.80    |
| beta1    | 0.67    |
| alpha2   | 6184.54 |
| beta2    | 6092.72 |
| P        | 0.38    |

The second gamma component degenerated to 1.

## Signals for FLU

| AE                              | N     | E        | RR   | PRR    | ebgm | ebgm_1 | ebgm_99 |
|---------------------------------|-------|----------|------|--------|------|--------|---------|
| Death                           | 6932  | 6517.61  | 1.06 | 5.32   | 1.05 | 1.02   | 1.09    |
| Vaccination site erythema       | 5822  | 5451.65  | 1.07 | 18.93  | 1.05 | 1.02   | 1.09    |
| Interchange of vaccine products | 8052  | 7620.54  | 1.06 | 222.50 | 1.04 | 1.02   | 1.07    |
| Vaccination site pain           | 12810 | 12155.00 | 1.05 | 6.68   | 1.04 | 1.02   | 1.07    |
| Vaccination site pruritus       | 3783  | 3530.67  | 1.07 | 52.27  | 1.04 | 1.01   | 1.10    |
| Chest pain                      | 18740 | 18171.65 | 1.03 | 3.23   | 1.03 | 1.01   | 1.04    |
| Condition aggravated            | 12335 | 11896.70 | 1.04 | 2.72   | 1.03 | 1.01   | 1.05    |
| Decreased appetite              | 10760 | 10434.79 | 1.03 | 1.93   | 1.03 | 1.01   | 1.04    |

| AE                                               | N      | E         | RR   | PRR   | ebgm | ebgm_1 | ebgm_99 |
|--------------------------------------------------|--------|-----------|------|-------|------|--------|---------|
| Fatigue                                          | 95114  | 91871.37  | 1.04 | 3.00  | 1.03 | 1.03   | 1.04    |
| Headache                                         | 113042 | 109755.94 | 1.03 | 2.46  | 1.03 | 1.02   | 1.04    |
| Inappropriate schedule of product administration | 6824   | 6494.88   | 1.05 | 13.47 | 1.03 | 1.01   | 1.06    |
| Lymphadenopathy                                  | 19611  | 18983.36  | 1.03 | 3.71  | 1.03 | 1.01   | 1.04    |
| Palpitations                                     | 13140  | 12742.24  | 1.03 | 3.06  | 1.03 | 1.01   | 1.04    |
| Tinnitus                                         | 12471  | 11995.02  | 1.04 | 4.59  | 1.03 | 1.01   | 1.05    |
| Arthralgia                                       | 38840  | 38032.34  | 1.02 | 1.65  | 1.02 | 1.01   | 1.03    |
| Chills                                           | 83152  | 81148.64  | 1.02 | 1.94  | 1.02 | 1.01   | 1.03    |
| Diarrhoea                                        | 21428  | 20873.18  | 1.03 | 1.79  | 1.02 | 1.01   | 1.04    |
| Dizziness                                        | 64576  | 63289.83  | 1.02 | 1.82  | 1.02 | 1.01   | 1.03    |
| Dyspnoea                                         | 36741  | 35898.74  | 1.02 | 1.80  | 1.02 | 1.01   | 1.03    |
| Feeling abnormal                                 | 19996  | 19452.20  | 1.03 | 2.07  | 1.02 | 1.01   | 1.04    |
| Myalgia                                          | 39142  | 38358.36  | 1.02 | 1.66  | 1.02 | 1.01   | 1.03    |
| Nausea                                           | 64408  | 63124.08  | 1.02 | 1.71  | 1.02 | 1.01   | 1.03    |
| Others                                           | 118917 | 116287.37 | 1.02 | 1.71  | 1.02 | 1.01   | 1.03    |
| Pyrexia                                          | 94454  | 93008.92  | 1.02 | 1.49  | 1.02 | 1.01   | 1.02    |

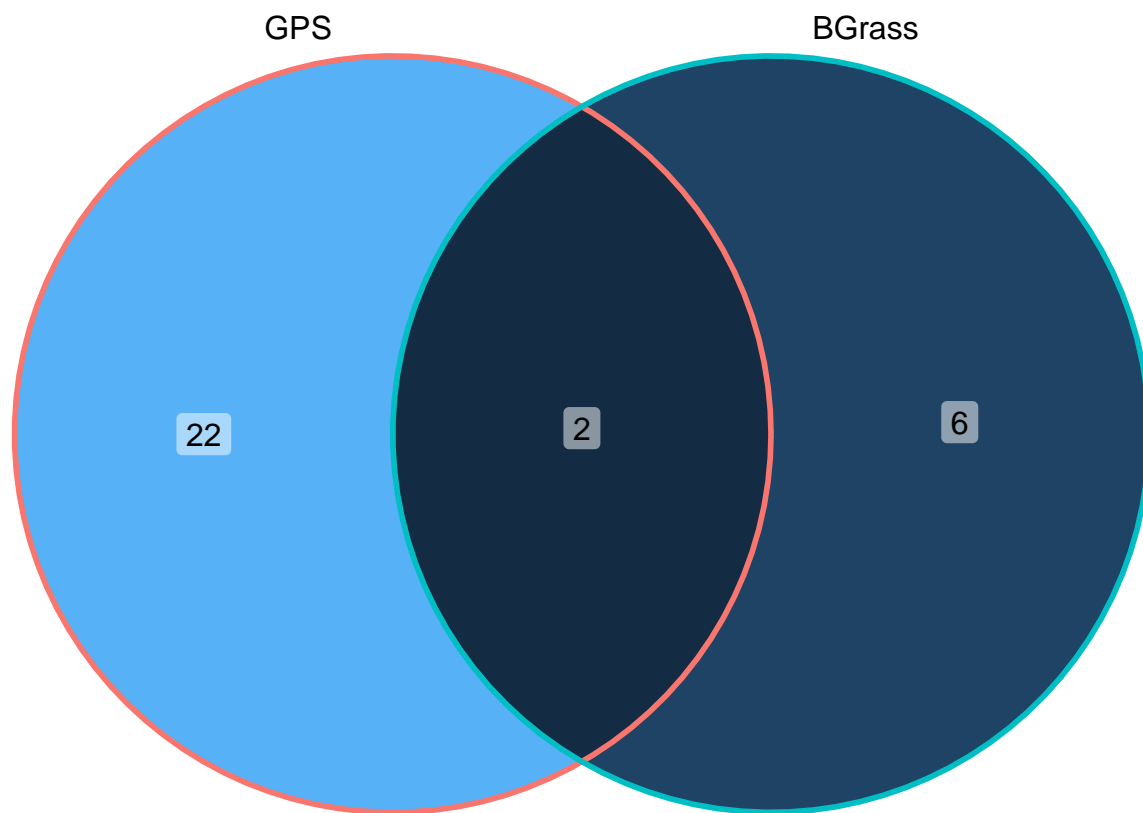

| AE                        | Model        |
|---------------------------|--------------|
| Vaccination site erythema | BGrass + GPS |
| Vaccination site pruritus | BGrass + GPS |
| Ageusia                   | BGrass       |
| Anosmia                   | BGrass       |

| AE                                               | Model  |
|--------------------------------------------------|--------|
| Deep vein thrombosis                             | BGrass |
| Menstruation disorder                            | BGrass |
| Pulmonary embolism                               | BGrass |
| Thrombosis                                       | BGrass |
| Arthralgia                                       | GPS    |
| Chest pain                                       | GPS    |
| Chills                                           | GPS    |
| Condition aggravated                             | GPS    |
| Death                                            | GPS    |
| Decreased appetite                               | GPS    |
| Diarrhoea                                        | GPS    |
| Dizziness                                        | GPS    |
| Dyspnoea                                         | GPS    |
| Fatigue                                          | GPS    |
| Feeling abnormal                                 | GPS    |
| Headache                                         | GPS    |
| Inappropriate schedule of product administration | GPS    |
| Interchange of vaccine products                  | GPS    |
| Lymphadenopathy                                  | GPS    |
| Myalgia                                          | GPS    |
| Nausea                                           | GPS    |
| Others                                           | GPS    |
| Palpitations                                     | GPS    |
| Pyrexia                                          | GPS    |
| Tinnitus                                         | GPS    |
| Vaccination site pain                            | GPS    |

## Study II

|        | Estimate |
|--------|----------|
| alpha1 | 3.92     |
| beta1  | 3.13     |
| alpha2 | 1113.18  |
| beta2  | 1128.58  |
| P      | 0.34     |

## Signals for mRNA-based Vaccines

| AE                                               | N     | E        | RR   | PRR   | ebgm | ebgm_1 | ebgm_99 |
|--------------------------------------------------|-------|----------|------|-------|------|--------|---------|
| Myocarditis                                      | 1537  | 1385.12  | 1.11 | 2.64  | 1.10 | 1.02   | 1.18    |
| Inappropriate schedule of product administration | 6721  | 6235.17  | 1.08 | 4.74  | 1.07 | 1.04   | 1.10    |
| Vaccination site pain                            | 12748 | 11872.12 | 1.07 | 19.34 | 1.07 | 1.04   | 1.09    |
| Injection site erythema                          | 26459 | 24991.91 | 1.06 | 4.44  | 1.06 | 1.04   | 1.07    |
| Injection site pruritus                          | 18573 | 17441.80 | 1.06 | 7.19  | 1.06 | 1.04   | 1.08    |
| Injection site rash                              | 10384 | 9723.25  | 1.07 | 7.56  | 1.06 | 1.04   | 1.09    |
| Injection site warmth                            | 13597 | 12812.31 | 1.06 | 4.74  | 1.06 | 1.04   | 1.08    |

| AE                           | N     | E        | RR   | PRR   | ebgm | ebgm_1 | ebgm_99 |
|------------------------------|-------|----------|------|-------|------|--------|---------|
| Lymphadenopathy              | 19083 | 17957.63 | 1.06 | 3.12  | 1.06 | 1.04   | 1.08    |
| Vaccination site swelling    | 4843  | 4534.19  | 1.07 | 31.49 | 1.06 | 1.02   | 1.10    |
| Axillary pain                | 5062  | 4767.86  | 1.06 | 3.07  | 1.05 | 1.02   | 1.09    |
| Injection site induration    | 5144  | 4852.02  | 1.06 | 4.26  | 1.05 | 1.01   | 1.09    |
| Injection site swelling      | 21526 | 20485.71 | 1.05 | 2.95  | 1.05 | 1.03   | 1.06    |
| Lymph node pain              | 4497  | 4237.87  | 1.06 | 3.08  | 1.05 | 1.01   | 1.09    |
| Product storage error        | 9014  | 8529.21  | 1.06 | 1.95  | 1.05 | 1.03   | 1.08    |
| Erythema                     | 20503 | 19727.36 | 1.04 | 2.32  | 1.04 | 1.02   | 1.05    |
| Injection site reaction      | 4236  | 4018.51  | 1.05 | 3.16  | 1.04 | 1.01   | 1.08    |
| Rash erythematous            | 9233  | 8840.08  | 1.04 | 2.49  | 1.04 | 1.01   | 1.06    |
| Expired product administered | 8869  | 8562.63  | 1.04 | 1.42  | 1.03 | 1.01   | 1.06    |
| Pruritus                     | 30176 | 29121.02 | 1.04 | 2.03  | 1.03 | 1.02   | 1.05    |
| Swelling                     | 10072 | 9695.72  | 1.04 | 2.04  | 1.03 | 1.01   | 1.06    |
| Rash                         | 31561 | 30891.84 | 1.02 | 1.42  | 1.02 | 1.01   | 1.03    |

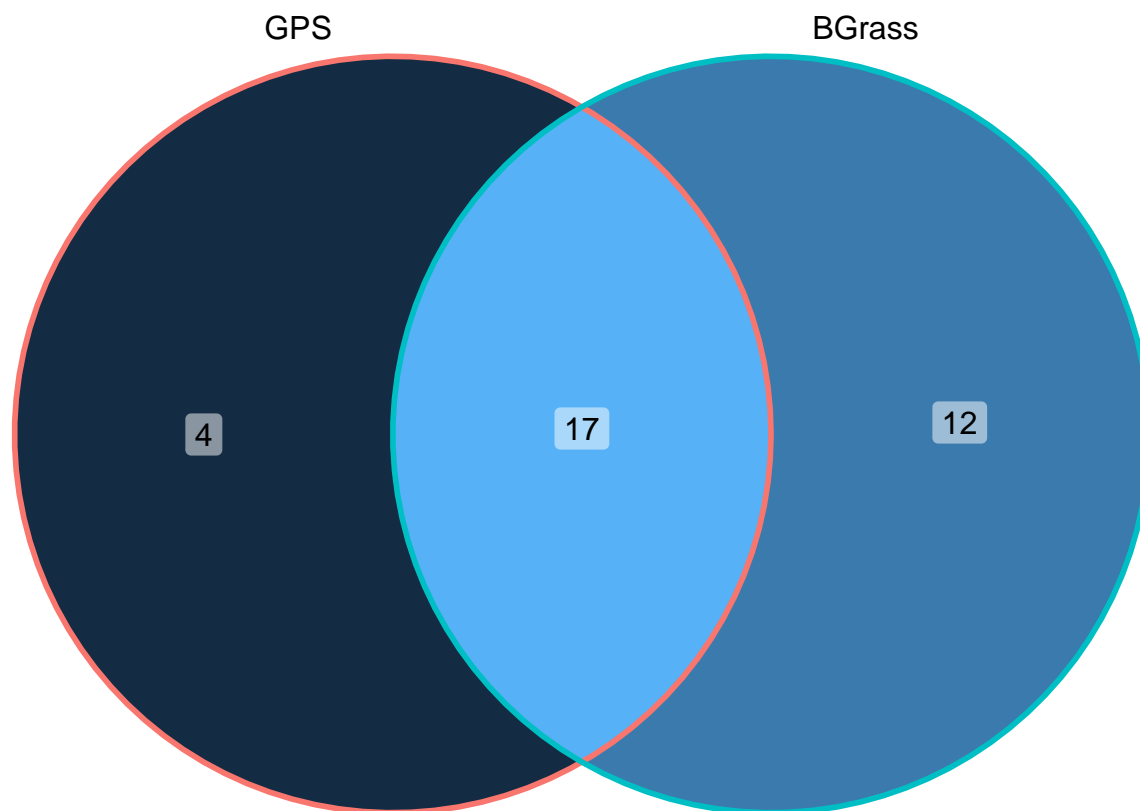

| AE                                               | Model        |
|--------------------------------------------------|--------------|
| Axillary pain                                    | BGrass + GPS |
| Erythema                                         | BGrass + GPS |
| Inappropriate schedule of product administration | BGrass + GPS |
| Injection site erythema                          | BGrass + GPS |
| Injection site induration                        | BGrass + GPS |
| Injection site pruritus                          | BGrass + GPS |
| Injection site rash                              | BGrass + GPS |

| AE                                         | Model        |
|--------------------------------------------|--------------|
| Injection site reaction                    | BGrass + GPS |
| Injection site swelling                    | BGrass + GPS |
| Injection site warmth                      | BGrass + GPS |
| Lymph node pain                            | BGrass + GPS |
| Lymphadenopathy                            | BGrass + GPS |
| Myocarditis                                | BGrass + GPS |
| Product storage error                      | BGrass + GPS |
| Rash erythematous                          | BGrass + GPS |
| Vaccination site pain                      | BGrass + GPS |
| Vaccination site swelling                  | BGrass + GPS |
| Axillary mass                              | BGrass       |
| Immunisation                               | BGrass       |
| Incorrect product formulation administered | BGrass       |
| Incorrect route of product administration  | BGrass       |
| Injection site inflammation                | BGrass       |
| Injection site urticaria                   | BGrass       |
| Lymphadenitis                              | BGrass       |
| Maternal exposure during pregnancy         | BGrass       |
| Rash papular                               | BGrass       |
| Skin reaction                              | BGrass       |
| Tongue pruritus                            | BGrass       |
| Vaccine positive rechallenge               | BGrass       |
| Expired product administered               | GPS          |
| Pruritus                                   | GPS          |
| Rash                                       | GPS          |
| Swelling                                   | GPS          |

## Signals for JJ

| AE                               | N   | E      | RR    | PRR   | ebgm | ebgm_1 | ebgm_99 |
|----------------------------------|-----|--------|-------|-------|------|--------|---------|
| Therapy non-responder            | 121 | 11.73  | 10.31 | 60.42 | 8.37 | 6.75   | 10.25   |
| Peripheral embolism              | 17  | 2.30   | 7.38  | 12.45 | 3.76 | 2.17   | 6.08    |
| On and off phenomenon            | 16  | 2.59   | 6.18  | 10.34 | 3.40 | 1.93   | 5.55    |
| Gaze palsy                       | 82  | 25.50  | 3.22  | 4.72  | 2.98 | 2.30   | 3.80    |
| Guillain-Barre syndrome          | 178 | 59.41  | 3.00  | 3.82  | 2.90 | 2.43   | 3.43    |
| Thrombophlebitis superficial     | 51  | 15.98  | 3.19  | 4.34  | 2.85 | 2.05   | 3.85    |
| Intracardiac thrombus            | 24  | 7.08   | 3.39  | 3.94  | 2.69 | 1.68   | 4.08    |
| Cerebral haemorrhage             | 74  | 25.85  | 2.86  | 2.72  | 2.67 | 2.03   | 3.45    |
| Deep vein thrombosis             | 472 | 177.21 | 2.66  | 3.07  | 2.64 | 2.37   | 2.93    |
| Varicose vein                    | 26  | 8.03   | 3.24  | 3.62  | 2.64 | 1.67   | 3.95    |
| Vasodilatation                   | 36  | 11.78  | 3.06  | 3.63  | 2.64 | 1.79   | 3.76    |
| Thrombosis                       | 675 | 256.45 | 2.63  | 2.94  | 2.61 | 2.39   | 2.86    |
| Portal vein thrombosis           | 24  | 7.53   | 3.19  | 4.55  | 2.57 | 1.60   | 3.91    |
| Embolic stroke                   | 14  | 3.86   | 3.63  | 3.58  | 2.47 | 1.03   | 4.18    |
| Mechanical ventilation           | 104 | 40.78  | 2.55  | 2.45  | 2.45 | 1.94   | 3.04    |
| Bilevel positive airway pressure | 33  | 12.01  | 2.75  | 2.34  | 2.41 | 1.60   | 3.47    |
| Thrombocytopenia                 | 115 | 46.26  | 2.49  | 2.53  | 2.40 | 1.93   | 2.95    |
| Transverse sinus thrombosis      | 16  | 4.89   | 3.27  | 4.29  | 2.40 | 1.14   | 3.95    |
| Immunoglobulin therapy           | 110 | 44.40  | 2.48  | 3.01  | 2.39 | 1.90   | 2.95    |
| Cerebral artery occlusion        | 17  | 5.52   | 3.08  | 3.52  | 2.34 | 1.10   | 3.82    |

| AE                                    | N    | E      | RR   | PRR  | ebgm | ebgm_1 | ebgm_99 |
|---------------------------------------|------|--------|------|------|------|--------|---------|
| Platelet transfusion                  | 30   | 11.17  | 2.68 | 2.82 | 2.34 | 1.52   | 3.42    |
| Posture abnormal                      | 72   | 29.34  | 2.45 | 3.42 | 2.32 | 1.76   | 3.01    |
| Pulmonary embolism                    | 542  | 233.33 | 2.32 | 2.51 | 2.31 | 2.09   | 2.55    |
| Pulmonary thrombosis                  | 101  | 42.13  | 2.40 | 2.47 | 2.31 | 1.83   | 2.87    |
| Overdose                              | 46   | 18.82  | 2.44 | 3.10 | 2.25 | 1.59   | 3.09    |
| Thrombectomy                          | 50   | 20.67  | 2.42 | 2.65 | 2.24 | 1.61   | 3.04    |
| Ischaemic stroke                      | 56   | 23.92  | 2.34 | 2.24 | 2.20 | 1.60   | 2.93    |
| Vaccination failure                   | 151  | 67.34  | 2.24 | 2.86 | 2.19 | 1.81   | 2.63    |
| Vein disorder                         | 27   | 10.86  | 2.49 | 2.97 | 2.17 | 1.36   | 3.24    |
| Hypoxia                               | 271  | 123.63 | 2.19 | 1.71 | 2.16 | 1.88   | 2.49    |
| Poor peripheral circulation           | 24   | 9.51   | 2.52 | 3.00 | 2.16 | 1.27   | 3.30    |
| Cerebral thrombosis                   | 30   | 12.59  | 2.38 | 2.35 | 2.12 | 1.37   | 3.11    |
| Foaming at mouth                      | 22   | 8.84   | 2.49 | 3.14 | 2.11 | 1.03   | 3.27    |
| Muscle contracture                    | 23   | 9.33   | 2.46 | 3.12 | 2.11 | 1.07   | 3.24    |
| Tension                               | 46   | 20.43  | 2.25 | 3.08 | 2.10 | 1.49   | 2.88    |
| Respiratory failure                   | 80   | 36.74  | 2.18 | 1.69 | 2.09 | 1.60   | 2.68    |
| Acute respiratory distress syndrome   | 29   | 12.57  | 2.31 | 2.07 | 2.06 | 1.29   | 3.04    |
| Subarachnoid haemorrhage              | 24   | 10.27  | 2.34 | 2.46 | 2.03 | 1.01   | 3.11    |
| Acute respiratory failure             | 184  | 89.83  | 2.05 | 1.58 | 2.02 | 1.69   | 2.38    |
| Urinary incontinence                  | 125  | 60.68  | 2.06 | 2.04 | 2.01 | 1.63   | 2.46    |
| Endotracheal intubation               | 161  | 79.21  | 2.03 | 1.84 | 2.00 | 1.66   | 2.39    |
| Sensory disturbance                   | 168  | 83.51  | 2.01 | 2.28 | 1.98 | 1.65   | 2.36    |
| Anticoagulant therapy                 | 317  | 159.51 | 1.99 | 2.05 | 1.97 | 1.72   | 2.24    |
| Haematemesis                          | 35   | 16.67  | 2.10 | 2.46 | 1.94 | 1.25   | 2.77    |
| Eye movement disorder                 | 162  | 82.68  | 1.96 | 2.93 | 1.93 | 1.60   | 2.30    |
| Intensive care                        | 284  | 145.50 | 1.95 | 1.89 | 1.93 | 1.68   | 2.21    |
| Contusion                             | 551  | 286.11 | 1.93 | 1.99 | 1.92 | 1.74   | 2.11    |
| Haemoptysis                           | 65   | 32.47  | 2.00 | 2.25 | 1.92 | 1.43   | 2.52    |
| Hemiparesis                           | 118  | 60.50  | 1.95 | 1.95 | 1.91 | 1.53   | 2.34    |
| Hypotonia                             | 41   | 20.38  | 2.01 | 2.68 | 1.89 | 1.28   | 2.64    |
| Incoherent                            | 42   | 20.86  | 2.01 | 2.12 | 1.89 | 1.30   | 2.63    |
| Cerebral infarction                   | 38   | 18.81  | 2.02 | 1.86 | 1.88 | 1.24   | 2.66    |
| Neurological symptom                  | 91   | 47.44  | 1.92 | 1.87 | 1.87 | 1.46   | 2.36    |
| Feeling cold                          | 1012 | 543.06 | 1.86 | 2.07 | 1.86 | 1.72   | 2.00    |
| Cerebrovascular accident              | 334  | 179.52 | 1.86 | 1.59 | 1.85 | 1.62   | 2.09    |
| Hemiplegia                            | 40   | 20.25  | 1.97 | 1.96 | 1.85 | 1.23   | 2.60    |
| Hypophagia                            | 65   | 34.04  | 1.91 | 1.60 | 1.84 | 1.37   | 2.42    |
| Restless legs syndrome                | 42   | 21.59  | 1.94 | 2.12 | 1.83 | 1.23   | 2.55    |
| Vision blurred                        | 1022 | 557.69 | 1.83 | 2.14 | 1.83 | 1.70   | 1.96    |
| General physical health deterioration | 62   | 32.90  | 1.88 | 1.37 | 1.82 | 1.34   | 2.39    |
| Rectal haemorrhage                    | 34   | 17.30  | 1.97 | 1.74 | 1.82 | 1.01   | 2.62    |
| Respiratory distress                  | 65   | 34.52  | 1.88 | 1.65 | 1.82 | 1.35   | 2.38    |
| Loss of consciousness                 | 1735 | 958.44 | 1.81 | 2.59 | 1.81 | 1.71   | 1.91    |
| Muscle spasms                         | 1128 | 632.02 | 1.78 | 1.96 | 1.78 | 1.66   | 1.91    |
| Fear of injection                     | 65   | 35.60  | 1.83 | 3.35 | 1.77 | 1.31   | 2.31    |
| Vaccine breakthrough infection        | 237  | 132.36 | 1.79 | 1.52 | 1.77 | 1.52   | 2.06    |
| Blindness unilateral                  | 51   | 27.68  | 1.84 | 1.83 | 1.76 | 1.24   | 2.39    |
| Groin pain                            | 67   | 37.01  | 1.81 | 1.90 | 1.75 | 1.31   | 2.29    |
| Pallor                                | 913  | 527.23 | 1.73 | 2.75 | 1.73 | 1.60   | 1.87    |
| Eye haemorrhage                       | 42   | 23.08  | 1.82 | 1.80 | 1.72 | 1.01   | 2.41    |
| Immediate post-injection reaction     | 814  | 471.77 | 1.73 | 2.04 | 1.72 | 1.59   | 1.87    |
| Renal pain                            | 100  | 57.50  | 1.74 | 2.07 | 1.71 | 1.35   | 2.13    |

| AE                                 | N    | E       | RR   | PRR  | ebgm | ebgm_1 | ebgm_99 |
|------------------------------------|------|---------|------|------|------|--------|---------|
| Spinal pain                        | 98   | 56.21   | 1.74 | 1.88 | 1.71 | 1.35   | 2.14    |
| Coordination abnormal              | 46   | 25.81   | 1.78 | 1.89 | 1.70 | 1.02   | 2.34    |
| Lung infiltration                  | 72   | 41.21   | 1.75 | 1.40 | 1.70 | 1.28   | 2.20    |
| Syncope                            | 2238 | 1320.95 | 1.69 | 2.49 | 1.69 | 1.61   | 1.78    |
| Petechiae                          | 101  | 58.95   | 1.71 | 1.91 | 1.68 | 1.33   | 2.10    |
| Injection site haemorrhage         | 66   | 38.46   | 1.72 | 1.78 | 1.67 | 1.23   | 2.18    |
| Abdominal pain                     | 860  | 519.61  | 1.66 | 1.76 | 1.65 | 1.53   | 1.78    |
| Head injury                        | 292  | 176.00  | 1.66 | 2.36 | 1.65 | 1.44   | 1.89    |
| Tremor                             | 1767 | 1069.61 | 1.65 | 1.82 | 1.65 | 1.56   | 1.74    |
| Blindness                          | 138  | 83.41   | 1.65 | 2.04 | 1.63 | 1.34   | 1.97    |
| Dysarthria                         | 191  | 115.95  | 1.65 | 1.65 | 1.63 | 1.38   | 1.92    |
| Transient ischaemic attack         | 73   | 43.62   | 1.67 | 1.46 | 1.63 | 1.22   | 2.11    |
| Abdominal pain lower               | 94   | 56.89   | 1.65 | 1.72 | 1.62 | 1.27   | 2.04    |
| Hyperhidrosis                      | 3318 | 2044.53 | 1.62 | 2.12 | 1.62 | 1.56   | 1.69    |
| Unresponsive to stimuli            | 623  | 383.57  | 1.62 | 2.21 | 1.62 | 1.47   | 1.78    |
| Dyspnoea exertional                | 158  | 97.14   | 1.63 | 1.65 | 1.61 | 1.34   | 1.93    |
| Hypotension                        | 511  | 316.44  | 1.61 | 1.89 | 1.61 | 1.45   | 1.78    |
| Mental status changes              | 99   | 60.44   | 1.64 | 1.22 | 1.61 | 1.27   | 2.01    |
| Thirst                             | 180  | 110.98  | 1.62 | 1.75 | 1.61 | 1.35   | 1.90    |
| Crying                             | 103  | 63.66   | 1.62 | 1.74 | 1.59 | 1.26   | 1.98    |
| Death                              | 655  | 411.08  | 1.59 | 1.14 | 1.59 | 1.45   | 1.74    |
| Fall                               | 882  | 556.17  | 1.59 | 1.84 | 1.58 | 1.46   | 1.71    |
| Feeling of body temperature change | 179  | 112.53  | 1.59 | 1.77 | 1.58 | 1.32   | 1.87    |
| Hyperaesthesia                     | 76   | 46.95   | 1.62 | 1.80 | 1.58 | 1.18   | 2.04    |
| Photophobia                        | 254  | 159.63  | 1.59 | 1.82 | 1.58 | 1.37   | 1.83    |
| Cold sweat                         | 606  | 383.95  | 1.58 | 2.06 | 1.57 | 1.43   | 1.73    |
| Eye pain                           | 370  | 234.46  | 1.58 | 1.65 | 1.57 | 1.39   | 1.77    |
| Sleep disorder                     | 1028 | 651.97  | 1.58 | 1.69 | 1.57 | 1.46   | 1.69    |
| Abdominal pain upper               | 848  | 543.08  | 1.56 | 1.60 | 1.56 | 1.44   | 1.69    |
| Haemoglobin decreased              | 130  | 82.48   | 1.58 | 1.35 | 1.56 | 1.27   | 1.90    |
| Mental impairment                  | 81   | 50.80   | 1.59 | 1.68 | 1.56 | 1.17   | 2.00    |
| Muscular weakness                  | 828  | 528.48  | 1.57 | 1.58 | 1.56 | 1.44   | 1.69    |
| Seizure like phenomena             | 70   | 43.73   | 1.60 | 2.17 | 1.56 | 1.04   | 2.03    |
| Muscle fatigue                     | 81   | 51.34   | 1.58 | 1.96 | 1.55 | 1.14   | 1.98    |
| Acute kidney injury                | 126  | 80.77   | 1.56 | 1.20 | 1.54 | 1.25   | 1.88    |
| Epistaxis                          | 268  | 173.39  | 1.55 | 1.68 | 1.54 | 1.33   | 1.77    |
| Nuclear magnetic resonance imaging | 1427 | 923.14  | 1.55 | 1.61 | 1.54 | 1.45   | 1.64    |
| Visual impairment                  | 476  | 309.00  | 1.54 | 1.74 | 1.54 | 1.38   | 1.71    |
| Dyskinesia                         | 151  | 97.84   | 1.54 | 1.76 | 1.53 | 1.26   | 1.84    |
| Off label use                      | 135  | 87.08   | 1.55 | 1.47 | 1.53 | 1.25   | 1.86    |
| Disorientation                     | 280  | 183.53  | 1.53 | 1.64 | 1.52 | 1.32   | 1.74    |
| Dysstasia                          | 283  | 185.60  | 1.52 | 1.43 | 1.52 | 1.32   | 1.74    |
| Paranasal sinus discomfort         | 112  | 73.35   | 1.53 | 1.70 | 1.51 | 1.20   | 1.86    |
| Restlessness                       | 124  | 81.50   | 1.52 | 1.72 | 1.51 | 1.21   | 1.84    |
| Resuscitation                      | 74   | 47.89   | 1.55 | 1.44 | 1.51 | 1.01   | 1.96    |
| Gait inability                     | 221  | 146.36  | 1.51 | 1.36 | 1.50 | 1.28   | 1.75    |
| Migraine                           | 1097 | 731.23  | 1.50 | 1.68 | 1.50 | 1.40   | 1.60    |
| Dehydration                        | 293  | 196.08  | 1.49 | 1.52 | 1.49 | 1.30   | 1.70    |
| Pneumonia                          | 237  | 158.96  | 1.49 | 1.22 | 1.48 | 1.27   | 1.72    |
| Seizure                            | 589  | 396.74  | 1.48 | 2.01 | 1.48 | 1.34   | 1.63    |
| Influenza like illness             | 1014 | 688.71  | 1.47 | 1.51 | 1.47 | 1.37   | 1.58    |
| Back pain                          | 1470 | 1007.30 | 1.46 | 1.50 | 1.46 | 1.37   | 1.55    |

| AE                                                | N     | E       | RR   | PRR  | ebgm | ebgm_1 | ebgm_99 |
|---------------------------------------------------|-------|---------|------|------|------|--------|---------|
| Gait disturbance                                  | 735   | 504.09  | 1.46 | 1.35 | 1.46 | 1.34   | 1.59    |
| Insomnia                                          | 894   | 611.40  | 1.46 | 1.55 | 1.46 | 1.35   | 1.58    |
| Hallucination                                     | 96    | 65.47   | 1.47 | 1.44 | 1.44 | 1.01   | 1.81    |
| Aphasia                                           | 174   | 121.39  | 1.43 | 1.37 | 1.42 | 1.19   | 1.69    |
| Skin discolouration                               | 241   | 170.02  | 1.42 | 1.40 | 1.41 | 1.21   | 1.63    |
| Headache                                          | 13230 | 9537.92 | 1.39 | 1.45 | 1.39 | 1.36   | 1.41    |
| Retching                                          | 161   | 114.73  | 1.40 | 1.34 | 1.39 | 1.14   | 1.66    |
| Confusional state                                 | 567   | 409.76  | 1.38 | 1.40 | 1.38 | 1.25   | 1.52    |
| Presyncope                                        | 384   | 278.45  | 1.38 | 1.77 | 1.38 | 1.22   | 1.55    |
| Amnesia                                           | 139   | 99.99   | 1.39 | 1.38 | 1.37 | 1.03   | 1.67    |
| Peripheral coldness                               | 189   | 138.11  | 1.37 | 1.42 | 1.36 | 1.13   | 1.60    |
| Chills                                            | 9449  | 7020.38 | 1.35 | 1.41 | 1.35 | 1.31   | 1.38    |
| Hot flush                                         | 419   | 308.99  | 1.36 | 1.47 | 1.35 | 1.21   | 1.52    |
| Asthenia                                          | 2678  | 2000.31 | 1.34 | 1.26 | 1.34 | 1.28   | 1.40    |
| Head discomfort                                   | 313   | 232.45  | 1.35 | 1.39 | 1.34 | 1.18   | 1.53    |
| Muscle tightness                                  | 234   | 174.52  | 1.34 | 1.46 | 1.34 | 1.13   | 1.55    |
| Decreased appetite                                | 1082  | 812.56  | 1.33 | 1.23 | 1.33 | 1.24   | 1.43    |
| Neuralgia                                         | 247   | 184.88  | 1.34 | 1.36 | 1.33 | 1.14   | 1.54    |
| Pyrexia                                           | 10747 | 8083.67 | 1.33 | 1.41 | 1.33 | 1.30   | 1.36    |
| Bone pain                                         | 223   | 167.97  | 1.33 | 1.28 | 1.32 | 1.10   | 1.54    |
| Dizziness                                         | 7639  | 5770.48 | 1.32 | 1.47 | 1.32 | 1.29   | 1.36    |
| Others                                            | 12986 | 9825.38 | 1.32 | 1.35 | 1.32 | 1.30   | 1.35    |
| Vomiting                                          | 2785  | 2114.88 | 1.32 | 1.38 | 1.32 | 1.26   | 1.37    |
| Hypoaesthesia                                     | 2355  | 1806.47 | 1.30 | 1.42 | 1.30 | 1.24   | 1.37    |
| Nausea                                            | 7038  | 5432.02 | 1.30 | 1.35 | 1.30 | 1.26   | 1.33    |
| Pain                                              | 9066  | 6992.91 | 1.30 | 1.35 | 1.30 | 1.27   | 1.33    |
| Balance disorder                                  | 362   | 280.14  | 1.29 | 1.20 | 1.29 | 1.13   | 1.46    |
| Facial paralysis                                  | 260   | 202.14  | 1.29 | 1.35 | 1.28 | 1.05   | 1.47    |
| Dyspnoea                                          | 3881  | 3062.47 | 1.27 | 1.30 | 1.27 | 1.22   | 1.31    |
| Night sweats                                      | 284   | 223.79  | 1.27 | 1.37 | 1.26 | 1.04   | 1.45    |
| Underdose                                         | 271   | 213.36  | 1.27 | 1.43 | 1.26 | 1.03   | 1.46    |
| Paraesthesia                                      | 2387  | 1913.85 | 1.25 | 1.34 | 1.25 | 1.19   | 1.31    |
| Lethargy                                          | 646   | 524.92  | 1.23 | 1.25 | 1.23 | 1.12   | 1.35    |
| Loss of personal independence in daily activities | 412   | 339.29  | 1.21 | 1.18 | 1.21 | 1.03   | 1.35    |
| Somnolence                                        | 547   | 452.25  | 1.21 | 1.16 | 1.21 | 1.07   | 1.33    |
| Impaired work ability                             | 623   | 517.14  | 1.20 | 1.34 | 1.20 | 1.08   | 1.32    |
| Mobility decreased                                | 809   | 675.74  | 1.20 | 1.14 | 1.20 | 1.10   | 1.30    |
| Feeling abnormal                                  | 1940  | 1632.41 | 1.19 | 1.18 | 1.19 | 1.13   | 1.25    |
| Feeling hot                                       | 1114  | 938.53  | 1.19 | 1.25 | 1.19 | 1.10   | 1.27    |
| Hypertension                                      | 554   | 467.84  | 1.18 | 1.13 | 1.18 | 1.03   | 1.30    |
| Neck pain                                         | 952   | 806.41  | 1.18 | 1.16 | 1.18 | 1.09   | 1.27    |
| Burning sensation                                 | 613   | 523.69  | 1.17 | 1.15 | 1.16 | 1.02   | 1.28    |
| Fatigue                                           | 9133  | 7848.83 | 1.16 | 1.17 | 1.16 | 1.13   | 1.19    |
| Cough                                             | 1737  | 1508.24 | 1.15 | 1.11 | 1.15 | 1.09   | 1.22    |
| Condition aggravated                              | 1123  | 979.77  | 1.15 | 1.10 | 1.14 | 1.04   | 1.23    |
| Diarrhoea                                         | 1876  | 1660.44 | 1.13 | 1.05 | 1.13 | 1.06   | 1.19    |
| Malaise                                           | 1638  | 1455.66 | 1.13 | 1.11 | 1.12 | 1.04   | 1.19    |
| Myalgia                                           | 3667  | 3268.06 | 1.12 | 1.13 | 1.12 | 1.07   | 1.16    |
| Pain in extremity                                 | 5045  | 4808.76 | 1.05 | 1.00 | 1.04 | 1.01   | 1.07    |



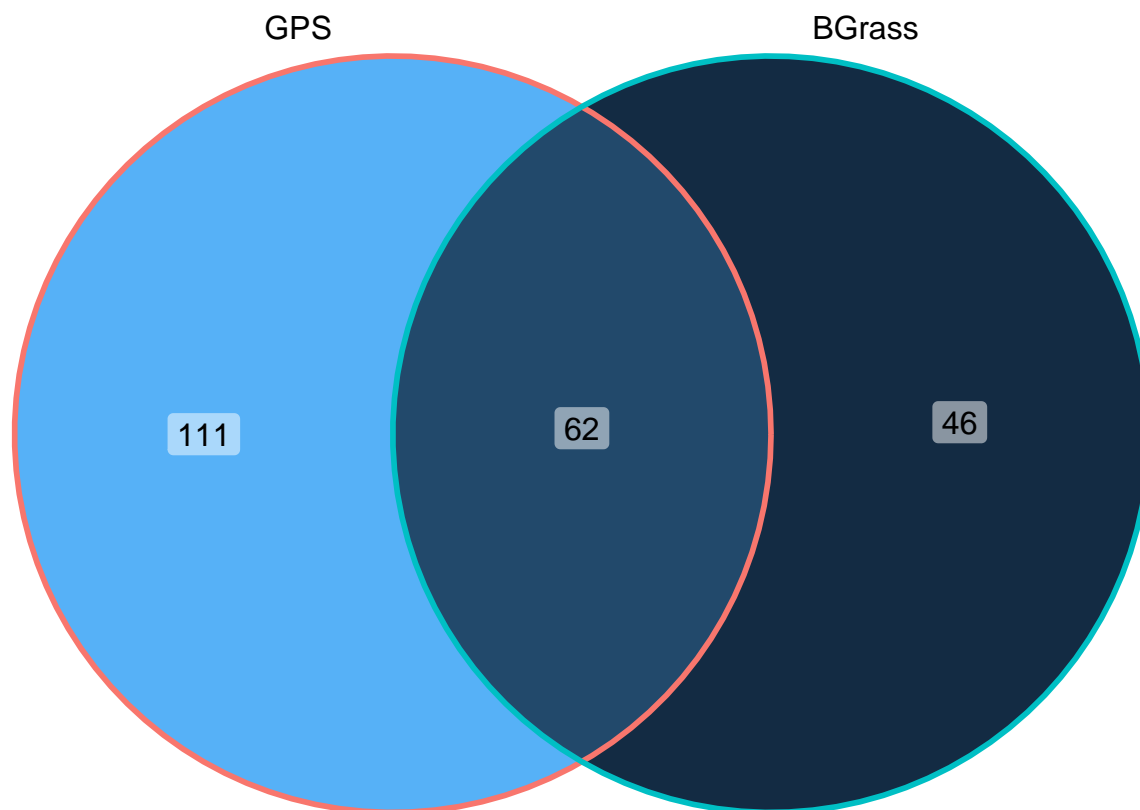

| AE                                  | Model        |
|-------------------------------------|--------------|
| Acute respiratory distress syndrome | BGrass + GPS |
| Acute respiratory failure           | BGrass + GPS |
| Anticoagulant therapy               | BGrass + GPS |
| Bilevel positive airway pressure    | BGrass + GPS |
| Cerebral artery occlusion           | BGrass + GPS |
| Cerebral haemorrhage                | BGrass + GPS |
| Cerebral infarction                 | BGrass + GPS |
| Cerebral thrombosis                 | BGrass + GPS |
| Cerebrovascular accident            | BGrass + GPS |
| Contusion                           | BGrass + GPS |
| Deep vein thrombosis                | BGrass + GPS |
| Embolic stroke                      | BGrass + GPS |
| Endotracheal intubation             | BGrass + GPS |
| Eye movement disorder               | BGrass + GPS |
| Fear of injection                   | BGrass + GPS |
| Feeling cold                        | BGrass + GPS |
| Foaming at mouth                    | BGrass + GPS |
| Gaze palsy                          | BGrass + GPS |
| Groin pain                          | BGrass + GPS |
| Guillain-Barre syndrome             | BGrass + GPS |
| Haematemesis                        | BGrass + GPS |
| Haemoptysis                         | BGrass + GPS |
| Hemiparesis                         | BGrass + GPS |
| Hypophagia                          | BGrass + GPS |

| AE                                                        | Model        |
|-----------------------------------------------------------|--------------|
| Hypotonia                                                 | BGrass + GPS |
| Hypoxia                                                   | BGrass + GPS |
| Immunoglobulin therapy                                    | BGrass + GPS |
| Incoherent                                                | BGrass + GPS |
| Intensive care                                            | BGrass + GPS |
| Intracardiac thrombus                                     | BGrass + GPS |
| Ischaemic stroke                                          | BGrass + GPS |
| Loss of consciousness                                     | BGrass + GPS |
| Mechanical ventilation                                    | BGrass + GPS |
| Muscle contracture                                        | BGrass + GPS |
| On and off phenomenon                                     | BGrass + GPS |
| Overdose                                                  | BGrass + GPS |
| Peripheral embolism                                       | BGrass + GPS |
| Platelet transfusion                                      | BGrass + GPS |
| Poor peripheral circulation                               | BGrass + GPS |
| Portal vein thrombosis                                    | BGrass + GPS |
| Posture abnormal                                          | BGrass + GPS |
| Pulmonary embolism                                        | BGrass + GPS |
| Pulmonary thrombosis                                      | BGrass + GPS |
| Rectal haemorrhage                                        | BGrass + GPS |
| Renal pain                                                | BGrass + GPS |
| Respiratory failure                                       | BGrass + GPS |
| Restless legs syndrome                                    | BGrass + GPS |
| Sensory disturbance                                       | BGrass + GPS |
| Subarachnoid haemorrhage                                  | BGrass + GPS |
| Tension                                                   | BGrass + GPS |
| Therapy non-responder                                     | BGrass + GPS |
| Thrombectomy                                              | BGrass + GPS |
| Thrombocytopenia                                          | BGrass + GPS |
| Thrombophlebitis superficial                              | BGrass + GPS |
| Thrombosis                                                | BGrass + GPS |
| Transverse sinus thrombosis                               | BGrass + GPS |
| Urinary incontinence                                      | BGrass + GPS |
| Vaccination failure                                       | BGrass + GPS |
| Varicose vein                                             | BGrass + GPS |
| Vasodilatation                                            | BGrass + GPS |
| Vein disorder                                             | BGrass + GPS |
| Vision blurred                                            | BGrass + GPS |
| Acute left ventricular failure                            | BGrass       |
| Affect lability                                           | BGrass       |
| Apathy                                                    | BGrass       |
| Atypical pneumonia                                        | BGrass       |
| Bladder catheterisation                                   | BGrass       |
| Capillary fragility                                       | BGrass       |
| Carotid artery occlusion                                  | BGrass       |
| Carotid artery stenosis                                   | BGrass       |
| Carotid artery thrombosis                                 | BGrass       |
| Cerebral small vessel ischaemic disease                   | BGrass       |
| Cerebral venous thrombosis                                | BGrass       |
| Chronic inflammatory demyelinating polyradiculoneuropathy | BGrass       |
| Coronary artery thrombosis                                | BGrass       |
| Craniocerebral injury                                     | BGrass       |

| AE                                 | Model  |
|------------------------------------|--------|
| Craniotomy                         | BGrass |
| Dysaesthesia                       | BGrass |
| Embolism                           | BGrass |
| Emphysema                          | BGrass |
| Extubation                         | BGrass |
| Fine motor skill dysfunction       | BGrass |
| Fluid intake reduced               | BGrass |
| Fluid replacement                  | BGrass |
| Gastrointestinal tube insertion    | BGrass |
| General symptom                    | BGrass |
| Haemorrhagic stroke                | BGrass |
| Haemorrhoids thrombosed            | BGrass |
| Increased tendency to bruise       | BGrass |
| Jugular vein thrombosis            | BGrass |
| Mesenteric vein thrombosis         | BGrass |
| Nail discolouration                | BGrass |
| New daily persistent headache      | BGrass |
| Peripheral artery thrombosis       | BGrass |
| Piloerection                       | BGrass |
| Plasmapheresis                     | BGrass |
| Pneumonia viral                    | BGrass |
| Psychomotor hyperactivity          | BGrass |
| Rhinalgia                          | BGrass |
| Sick relative                      | BGrass |
| Snoring                            | BGrass |
| Spider vein                        | BGrass |
| Superior sagittal sinus thrombosis | BGrass |
| Thrombophlebitis                   | BGrass |
| Tracheostomy                       | BGrass |
| Type 2 diabetes mellitus           | BGrass |
| Urinary retention                  | BGrass |
| Venous occlusion                   | BGrass |
| Abdominal pain                     | GPS    |
| Abdominal pain lower               | GPS    |
| Abdominal pain upper               | GPS    |
| Acute kidney injury                | GPS    |
| Amnesia                            | GPS    |
| Aphasia                            | GPS    |
| Asthenia                           | GPS    |
| Back pain                          | GPS    |
| Balance disorder                   | GPS    |
| Blindness                          | GPS    |
| Blindness unilateral               | GPS    |
| Bone pain                          | GPS    |
| Burning sensation                  | GPS    |
| Chills                             | GPS    |
| Cold sweat                         | GPS    |
| Condition aggravated               | GPS    |
| Confusional state                  | GPS    |
| Coordination abnormal              | GPS    |
| Cough                              | GPS    |
| Crying                             | GPS    |

| AE                                                | Model |
|---------------------------------------------------|-------|
| Death                                             | GPS   |
| Decreased appetite                                | GPS   |
| Dehydration                                       | GPS   |
| Diarrhoea                                         | GPS   |
| Disorientation                                    | GPS   |
| Dizziness                                         | GPS   |
| Dysarthria                                        | GPS   |
| Dyskinesia                                        | GPS   |
| Dyspnoea                                          | GPS   |
| Dyspnoea exertional                               | GPS   |
| Dysstasia                                         | GPS   |
| Epistaxis                                         | GPS   |
| Eye haemorrhage                                   | GPS   |
| Eye pain                                          | GPS   |
| Facial paralysis                                  | GPS   |
| Fall                                              | GPS   |
| Fatigue                                           | GPS   |
| Feeling abnormal                                  | GPS   |
| Feeling hot                                       | GPS   |
| Feeling of body temperature change                | GPS   |
| Gait disturbance                                  | GPS   |
| Gait inability                                    | GPS   |
| General physical health deterioration             | GPS   |
| Haemoglobin decreased                             | GPS   |
| Hallucination                                     | GPS   |
| Head discomfort                                   | GPS   |
| Head injury                                       | GPS   |
| Headache                                          | GPS   |
| Hemiplegia                                        | GPS   |
| Hot flush                                         | GPS   |
| Hyperaesthesia                                    | GPS   |
| Hyperhidrosis                                     | GPS   |
| Hypertension                                      | GPS   |
| Hypoaesthesia                                     | GPS   |
| Hypotension                                       | GPS   |
| Immediate post-injection reaction                 | GPS   |
| Impaired work ability                             | GPS   |
| Influenza like illness                            | GPS   |
| Injection site haemorrhage                        | GPS   |
| Insomnia                                          | GPS   |
| Lethargy                                          | GPS   |
| Loss of personal independence in daily activities | GPS   |
| Lung infiltration                                 | GPS   |
| Malaise                                           | GPS   |
| Mental impairment                                 | GPS   |
| Mental status changes                             | GPS   |
| Migraine                                          | GPS   |
| Mobility decreased                                | GPS   |
| Muscle fatigue                                    | GPS   |
| Muscle spasms                                     | GPS   |
| Muscle tightness                                  | GPS   |
| Muscular weakness                                 | GPS   |

| AE                                 | Model |
|------------------------------------|-------|
| Myalgia                            | GPS   |
| Nausea                             | GPS   |
| Neck pain                          | GPS   |
| Neuralgia                          | GPS   |
| Neurological symptom               | GPS   |
| Night sweats                       | GPS   |
| Nuclear magnetic resonance imaging | GPS   |
| Off label use                      | GPS   |
| Others                             | GPS   |
| Pain                               | GPS   |
| Pain in extremity                  | GPS   |
| Pallor                             | GPS   |
| Paraesthesia                       | GPS   |
| Paranasal sinus discomfort         | GPS   |
| Peripheral coldness                | GPS   |
| Petechiae                          | GPS   |
| Photophobia                        | GPS   |
| Pneumonia                          | GPS   |
| Presyncope                         | GPS   |
| Pyrexia                            | GPS   |
| Respiratory distress               | GPS   |
| Restlessness                       | GPS   |
| Resuscitation                      | GPS   |
| Retching                           | GPS   |
| Seizure                            | GPS   |
| Seizure like phenomena             | GPS   |
| Skin discolouration                | GPS   |
| Sleep disorder                     | GPS   |
| Somnolence                         | GPS   |
| Spinal pain                        | GPS   |
| Syncope                            | GPS   |
| Thirst                             | GPS   |
| Transient ischaemic attack         | GPS   |
| Tremor                             | GPS   |
| Underdose                          | GPS   |
| Unresponsive to stimuli            | GPS   |
| Vaccine breakthrough infection     | GPS   |
| Visual impairment                  | GPS   |
| Vomiting                           | GPS   |
